# Supplementary material for: Enhancing Profit and CO2 Mitigation: Commercial Direct Air Capture Design and Operation with Power Market Volatility
Source: arXiv:2510.12949 source file (2025-10-14)
Supplement: Supplementary file 1 [file DAC_power_appendix_ArXiv_version.pdf]

# Enhancing Profit and $CO_2$ Mitigation: Commercial Direct Air Capture Design and Operation with Power Market Volatility – Supplementary Information

Zhiyuan Fan[1,2*], Elizabeth Dentzer[3], James Glynn[4], David S. Goldberg[5], Julio Friedmann[6], Bolun Xu[1*]

[1*]Earth and Environmental Engineering, Columbia University, 500 W. 120th Street #510, New York, 10027, NY, US.
[2*]Center on Global Energy Policy, Columbia University, 1255 Amsterdam Avenue, New York, 10027, NY, US.
[3]Department of Mechanical and Aerospace Engineering, Princeton University, NJ 084540, US.
[4]Energy Systems Modelling Analytics Limited, Galway, Ireland.
[5]Lamont-Doherty Earth Observatory, Columbia University, 61 Rte 9W, Palisades, New York, 10964, NY, US.
[6]Carbon Direct, 17 State Street, New York, 10004, NY, US.

*Corresponding author(s). E-mail(s): zf2198@columbia.edu; bx2177@columbia.edu;
Contributing authors: bd3796@princeton.edu; james@esma.ie; goldberg@ldeo.columbia.edu; jfriedmann@carbon-direct.com;

## 1 Methodology: Extended

In this section, a more detailed version of the methodology for DAC operation optimization is presented, including all constraints for the mixed-integer linear programming (MILP) optimization model written in Julia, and the custom *strategic bidding algorithm* algorithm written in MATLAB for cyclic DAC used for MOF, APDES-NFC-FD, and SI-AEATPMS. An MILP optimization model simulating the KOH liquid solvent continuous operation methodology is also included.

### 1.1 MILP for Cyclic DACs

The mixed-integer linear programming (MILP) is a rigorous optimization formulation for linearizing and solving inherently nonlinear and nonconvex process models. While MILP provides accurate profit-maximization results with optimality-bound guarantees, it is computationally expensive and practically unsolvable for technologies with long cycling periods or long optimization horizons.

Indexes:

- $t$: Time period index $t \in \{1, 2, ..., T\}$, a total of T time periods in optimization horizon.

Binary decision variables:

- $u_t$: 1 if DAC is during the absorption phase at time period $t$, otherwise zero.
- $v_t$: 1 if DAC is during the desorption phase at time period $t$, otherwise zero.
- $z_t$: 1 if DAC is switched to a new cycle at time period $t$, otherwise zero
- $k_t$: introduce new sign-variable to determine the change of status at time period $t$ to facilitate calculation of $z_t$

Continuous decision variables:

- $X_t$: state-of-saturation capacity of DAC system at time period $t$
- $a_t$: absorption amount of DAC system at time period $t$
- $d_t$: desorption amount of DAC system at time period $t$

System input parameters:

- $\lambda_t$: electricity price at time period $t$, can subjected to modification of $CO_2$ (see $\lambda e_t$)
- $e_t$: electricity $CO_2$-intensity at time period $t$
- $\rho_e$: $CO_2$ value of carbon for electricity, 0 if for wholesale electricity price case, $\pi$ if for carbon-tax adjusted electricity price case.
- $\lambda e_t$: electricity price without $CO_2$-intensity correction ($\lambda_t = \lambda e_t + \rho_e e_t$)
- $\eta_t$: adsorption rate correction factor at time period $t$, which is a function of relative humidity and temperature.
- $C_t$: energy consumption correction factor at time period $t$, which is a function of relative humidity and temperature.
- $\pi$: $CO_2$ value constant including selling price, subsidies, carbon-tax, etc.

DAC input parameters:

- $P^a$: electricity consumption for absorption phase per unit time period
- $P^d$: electricity consumption for desorption phase per unit time period
- $\bar{X}$: max available DAC capacity
- $S$: switching cycle cost for consumption of sorbent materials

Piecewise linear approximation for absorption/desorption rate using quadratic coefficients:

- $\beta_1^a$: first-order coefficient for absorption
- $\beta_2^a$: second-order coefficient for absorption
- $\beta_1^d$: first-order coefficient for desorption
- $\beta_2^d$: second-order coefficient for desorption

The objective function maximizes the total profit of the DAC operation.

$$max \sum_t \pi d_t - \lambda_t C_t (P^a u_t + P^d v_t) - S z_t \tag{1}$$

where $\pi d_t$ is the total revenue by captured (desorbed) $CO_2$, minus the cost of power consumption corrected by ambient conditions at each time step $\lambda_t C_t (P^a u_t + P^d v_t)$, minus the cost of material consumption for switching cycles $S z_t$.

Binary constraints for absorption/desorption status:

$$u_t + v_t \leq 1 \tag{2}$$

where the DAC system can only be adsorption/desorption at one time period, it can be neither absorbing nor desorbing.

Absorption and desorption rate (using inequality here to avoid contradiction with binary constraints, which is relaxation of the constraints), be mindful that only adsorption (capture) process is corrected by ambient condition of each time step, desorption is a controlled process which is not affected by ambient condition:

$$a_t \leq \eta_t^a (\beta_1^a + \beta_2^a X_t) \tag{3}$$

$$d_t \leq \beta_1^d + \beta_2^d X_t \tag{4}$$

additionally, the absorption rate and desorption rate shall be bounded by the binary variable for each as well.

$$a_t \leq M u_t \tag{5}$$

$$d_t \leq M v_t \tag{6}$$

where $M$ is a sufficiently large number which does not bind the absorption and desorption rate if $u_t$ and $v_t$ are 1.

Be careful that although the below constraints are not required to be added explicitly, they shall be automatically satisfied with the above absorption and desorption rate constraints:

$$0 \leq a_t \leq a_{max} \quad (7)$$

$$0 \leq d_t \leq d_{max} \quad (8)$$

where absorption and desorption rates are always bounded by 0 and its maximum designed capacity

State-of-saturation capacity of DAC system updates with absorption/desorption rates:

$$X_t - X_{t-1} = a_t - d_t \quad (9)$$

where the change of state-of-saturation between time periods equals: adding absorption; subtracting desorption. Both absorption and desorption are corrected by the binary decision variables.

$$0 \leq X_t \leq \bar{X} \quad (10)$$

where the state-of-saturation is always lower bounded by 0, and upper bounded by its maximum capacity $\bar{X}$

Switching cycle constraints:

$$k_0 = 0 \quad (11)$$

where the initial state of the sign-variable equals zero.

$$-M(1 - k_t) \leq k_{t-1} + (u_t - v_t) - 0.5 \quad (12)$$

$$Mk_t \geq k_{t-1} + (u_t - v_t) - 0.5 \quad (13)$$

where the sign function is defined here with a sufficiently large $M$. The comparison is subtracted by 0.5 to avoid the possible case that $k_{t-1} + (u_t - v_t) = 0$. The solution matrix for $k_t$ for all possible combinations of sign-function is given in below table:

| Variables | $k_{t-1} = 0$ | $k_{t-1} = 1$ |
|---|---|---|
| $u_t - v_t$ = -1 | 0 | 0 |
| $u_t - v_t = 0$ | 0 | 1 |
| $u_t - v_t = 1$ | 1 | 1 |

The above two equations together define the sign-variable $k_t$ which is used to determine the binary cycle counting variable $z_t$:

$$z_t \geq k_t - k_{t-1} \quad (14)$$

where $z_t$ will be minimized in the objective function that only when $k_t = 1$ and $k_{t-1} = 0$, $z_t = 1$.

The above formulation summarizes the optimization framework of the DAC system using the temperature-swing DAC technology (all 3 DAC technologies tested in this paper). In practice, the DAC input parameters including the piecewise linear approximation for absorption and desorption rate using quadratic coefficients will be determined by different DAC specifications. The actual optimization programs use a look-ahead framework (similar concept of MPC control) which looks longer optimization horizon but applies only the first few steps for action.

## 1.2 Custom Algorithm

A threshold-based formulation is rooted in a custom *strategic bidding* MATLAB algorithm, specifically designed to handle nonlinear processes. By participating in electricity markets through the bidding process, DAC operators can strategically operate during the low-price periods: activate operation if prices are lower than the threshold and idle if higher, hence mimicking market clearing of flexible demand bids, potentially generating more profit at market price valleys. The optimization problem is therefore greatly simplified to optimizing only 1 variable, the price threshold for each optimization horizon, increasing the computational efficiency.

The operation of the DAC follows exactly the same formulation as MILP, with additional key terms in this formulation including:

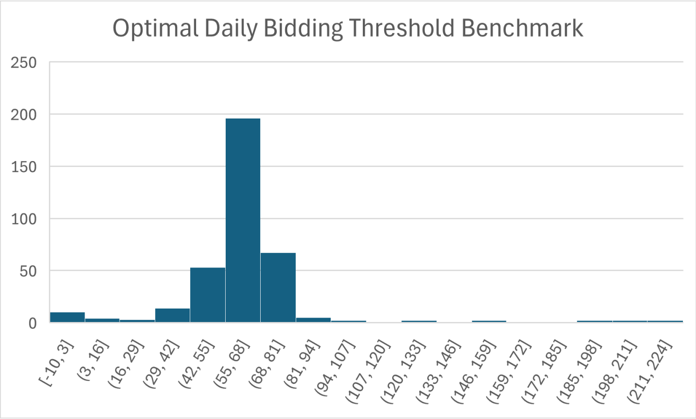


**Fig. S1**: Optimal bidding threshold robustness analysis based on MOF technology operating in CAISO power market for 365 consecutive days, median threshold adopted \$61.7/MWh.

- $\lambda_{\text{opt}}$: The price threshold, or the electricity price at which DAC operators are willing to operate.
- $c$: A data "chunk" for processing. Each chunk is optimized individually.

A typical chunk size $c$ is 24 hours, equivalent to 288 time steps (5-min temporal resolution), reflecting daily market price behaviors. However, the algorithm is designed with flexibility, allowing for adjustments in chunk size to cater to different market dynamics or operational needs for different DAC cycle times.

The DAC system's operation is determined by the threshold, $\lambda_{\text{opt}}$. The decision to either accept or reject is defined as:

$$\begin{cases} \text{Activate} & \text{if } \lambda_t(t) \leq \lambda_{\text{opt}} \\ \text{Idle} & \text{otherwise} \end{cases}$$

For each chunk $c$, the algorithm employs an iterative process to find the optimal $\lambda_{\text{opt}}$ that maximizes profit. It utilizes MATLAB's `fminsearch` function, which optimizes 1 variable to find the minimum of the objective function. Specifically, `fminsearch` is tasked to find the value of $\lambda_{\text{opt}}$ that minimizes the negative profit objective function, effectively maximizing profit.

To circumvent the issue of local minima and to ensure identification of the global minimum, the algorithm iterates over a series of initial guesses $\lambda_{\text{series}}$ for $\lambda_{\text{opt}}$ in the range from -10 to 500 USD. One may increase the granularity of the initial guesses to get a marginally better objective with a computation time trade-off. For each initial guess in the $\lambda_{\text{series}}$, `fminsearch` conducts an optimization to locate a local maximum. Upon the completion of all such iterations, the algorithm chooses the highest profit from these local maxima as the global maximum. This approach reduces the risk of the optimization process settling for a suboptimal local maximum.

The final determination of $\lambda^*_{\text{opt}}$ involves selecting the optimal value that corresponds to the maximum profit achieved across all the local optimizations:

$$\lambda^*_{\text{opt}} = \max_{\lambda_{\text{series}}} \text{fminsearch}(-\text{Objective}(c, \lambda_{\text{guess}})). \tag{15}$$

The max function in the equation is a representation of the selection process that identifies the highest value from all the local maxima obtained by `fminsearch`, starting from different initial guesses within the series. This comprehensive exploration across a diverse set of starting points helps in ensuring that the resulting $\lambda^*_{\text{opt}}$ is the most favorable for maximizing profit.

### 1.2.1 Look-Ahead Mechanism:

- $L$: Look-ahead parameter representing the number of future data points considered during optimization.
- $t$: Starting time of the given chunk $c$.

For a given chunk $c$ starting at time $t$, the algorithm factors in data from $t$ to $t + L$ to find the optimal $\lambda_{\text{opt}}$. The optimization process employs the MATLAB function `fminsearch`:

$$\lambda^*_{\text{opt}} = \text{fminsearch}(-\text{Objective}(c, \lambda_{\text{opt}}, L)) \tag{16}$$

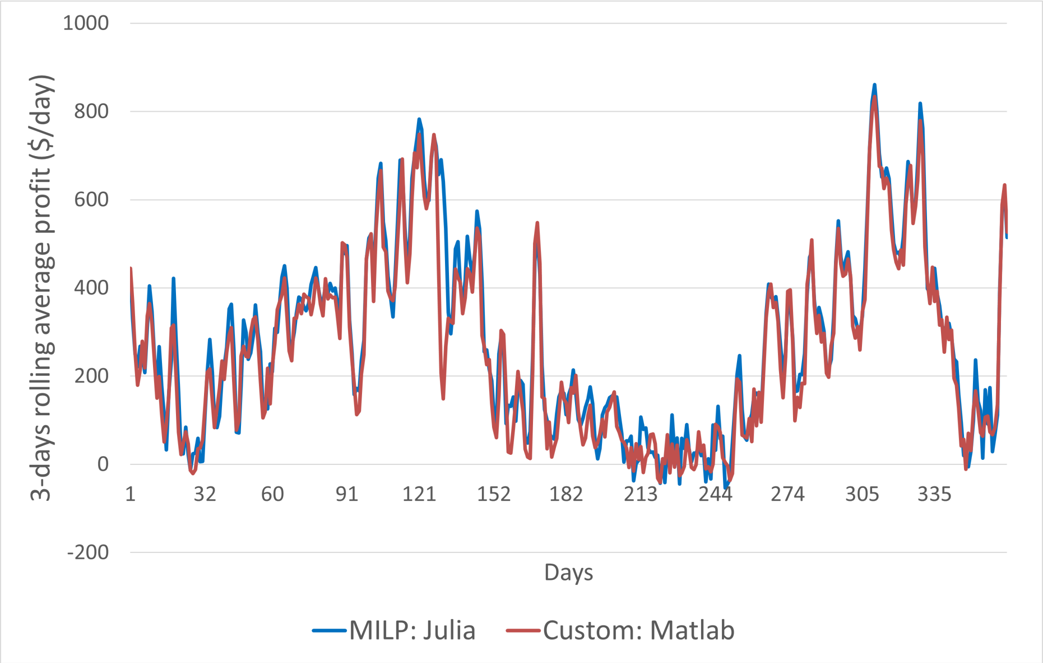


**Fig. S2**: **3-days rolling average profit for MILP and Custom algorithm optimality comparison in NY.** based on MOF technology, incentive selling price = \$200/ton-$CO_2$ . It shows that the customer algorithm pertains the optimality of rigurous MILP optimization method.

Where:

$$\text{Objective}(c, \lambda_{\text{opt}}, L)$$

is the profit obtained for chunk $c$ when using threshold $\lambda_{\text{opt}}$and considering $L$ future data points.

### 1.2.2 Boost Mechanism:

- **X_remain**: State-of-saturation at the end of the processed chunk. This represents the amount of $CO_2$ credit still in the system that hasn't been cleared yet.
- **Profit_chunk**: Total profit from the processed chunk.
- **CO2_chunk**: Total amount of $CO_2$ desorbed during the processed chunk

The boost mechanism is introduced to account for the potential value of the remaining $CO_2$ in the system at the end of the DAC loop to avoid selling all CO2 at the end of each chunk to maximize profit, which will force the DAC operation to terminate at the end of each optimization horizon. The boost is calculated using the following formula:

$$\text{boost} = \left(\frac{\text{Profit\_chunk}}{\text{CO2\_chunk}}\right) \times \text{X\_remain}$$

Where:

- $\frac{\text{Profit\_chunk}}{\text{CO2\_chunk}}$ represents the average profit per unit of $CO_2$ sold during the processed chunk. It indicates the expected value or profit obtained from selling one unit of $CO_2$.

After calculating the boost, it's added to the profit for that chunk. This accounts for both the profit from the $CO_2$ that was sold and the potential value of the $CO_2$ that remains in the system:

$$\text{Profit\_total} = \text{Profit\_chunk} + \text{boost}$$

However, it's important to note that this inflated profit is not used when calculating the overall profits. It is solely used for the process of finding the optimal lambda. This ensures that the optimization process considers both actual and potential profits, valuing scenarios where there's a significant amount of $CO_2$ left in the system at the end of the loop.

**Table S1**: Comparison of performances for MILP and Custom algorithm

| Case | Model | Execution Time (HH:MM:SS) | Profit ($) | Net CO2 Removal (Metric Tons) |
|---|---|---|---|---|
| NY Real-time Price | MILP | 07:57:04 | 102,557 | 2,555 |
| | Custom | 00:00:12 | 94,942 | 2,919 |
| | Comparison | 2,385× faster | −7.4% diff | 14.2% diff |
| NY Carbon-tax Price | MILP | 06:01:5 | 4,585 | 381 |
| | Custom | 00:00:12 | 3,035 | 342 |
| | Comparison | 1,809× faster | −33.8% diff | −10.2% diff |
| CA Real-time Price | MILP | 05:11:22 | 172,615 | 2,133 |
| | Custom | 00:00:15 | 153,491 | 2,408 |
| | Comparison | 1,245× faster | −11.1% diff | 12.9% diff |
| CA Carbon-tax Price | MILP | 03:03:46 | 93,793 | 1,283 |
| | Custom | 00:00:12 | 82,857 | 1,443 |
| | Comparison | 919× faster | −11.7% diff | 12.4% diff |
| TX Real-time Price | MILP | 07:48:14 | 134,061 | 2,599 |
| | Custom | 00:00:09 | 127,312 | 2,982 |
| | Comparison | 3,122× faster | −5.0% diff | 14.7% diff |
| TX Carbon-tax Price | MILP | 04:36:32 | 14,680 | 706 |
| | Custom | 00:00:10 | 13,170 | 804 |
| | Comparison | 1,844× faster | −10.3% diff | 13.9% diff |

*Note: based on MOF technology, incentive selling price = $200/ton-$CO_2$, carbon-tax value = $200/ton-$CO_2$ if applied.

## 1.3 Computational Performance Comparison

As shown in Table S1 and Figure S2, the Custom algorithm based on simplified price threshold preserves the MILP optimality with approximately 10% profit loss, but delivering more $CO_2$ removal in most cases and runs thousands times faster. The biggest profit optimality gap reported is NY case with carbon-tax while the profit is virtually close to zero, meaning the Custom algorithm is reliable across wide ranges of objective values. The trade-off between profit and net $CO_2$ removal is again proving the profitability is very sensitive to operation at certain periods. In practice, following 5-minute real-time pricing is very hard and mostly unachievable as it's highly uncertain and hard to predict. The custom algorithm with price threshold based on day-ahead pricing predictions will be more practical.

## 1.4 Computing Environment

The simulation results presented in this study were generated using a workstation with the following specifications:

- **Processor:** Intel® Core™ i9-12900H, 12th Gen (14 cores, 20 threads), base speed 2.50 GHz
- **Memory:** 64 GB RAM
- **Storage:** NVMe SSD
- **GPU:** NVIDIA RTX A2000 8GB (not utilized for optimization)
- **Operating System:** Windows 11 Pro
- **Solver:** *[Specify solver here, e.g., Gurobi 10.0 with Python API or MATLAB Optimization Toolbox]*

Under this configuration, a 1-year rolling-horizon optimization typically required **4–8 hours** for the cyclic DAC model and **1.5–2 hours** for the continuous model. Runtimes may vary depending on solver settings, model complexity, and machine load. Performance could be significantly improved using dedicated servers or high-performance computing clusters.

## 1.5 MILP for Continuous DACs

Modeling of the continuous DAC operation. The objective maximize the total profit of the DAC operation. The variables definition is consistent with the continuous DAC MILP setttings.

$$max \sum_t \pi d_t \eta_t^a - \lambda_t P_t^d - S_c d_t \tag{17}$$

where $\pi d_t$ is the total revenue corrected by ambient environment conditions $\eta_t^a$ minus the cost of power consumption $\lambda_t(P^a u_t + P^d v_t)$ and operational cost $S_c d_t$ which include both heat thermal energy cost and material consumption.

For continuous DAC, the operational flexiblity is determined by two constraints. The first one is ON/OFF limit constraints:

$$y_t - z_t = w_t - w_{t-1} \tag{18}$$

$$y_t - z_t \leq 1 \tag{19}$$

where $w_t$ is the binary on/off status of DAC, $y_t$ and $z_t$ indicating switching on and off status of DAC.

$$\sum_{\tau=1}^{I} (y_\tau + z_\tau) \leq K \tag{20}$$

meaning the total times of switching on or off during the horizon $(i \in 1, 2, ..., I)$ is limited by maximum flexibility index $K$. In practice, $I = 288$ 5-min time-steps, meaning the continuous DAC can maximum turn on/off by $K$ times in one day.

The second one is min/max rate constraints while turned on:

$$\underline{d} w_t \leq d_t \leq \bar{d} w_t \tag{21}$$

the capture rate of $CO_2$ $d_t$ is limited to 80% to 100% of maximum capture rate $\bar{d}$ whiled turned on, this is a typical way for flexibility testing from other industrial examples, such as aluminium [Depree et al., 2022] or hydrogen [Wang et al., 2018]. The 80% range is representative and should be tailor for each different technology. Accompanied with the power consumption constraints:

$$P_t^d = \frac{d_t}{\bar{d}} \bar{P}^t \tag{22}$$

where the actual power consumption $P_t^d$ is the fraction of nominal power consumption for capture $\bar{P}^t$.

The computational performance of continuous DAC MILP optimization is better than cyclic DAC, taking about 1.5 hours for a full year simulation under various assumptions of $K$. The optimization results are therefore determined by the setting of $K$ which fundamentally discribs the flexibility of DAC operation, whose impact is shown below.

## 1.6 Ambient correction calculations

Assuming all DAC nominal capacity and power consumption is measured under standard lab environment with baseline temperature of 20 °C and relative humidity of 50%. We applied the ambient sensitivity from two studies: [1] for cyclic DAC operation based on steam-assisted vacuum-pressure temperature swing adsorption with amine-functionalized solid sorbent; and [2] for continuous liquid solvent KOH DAC.

For cyclic DAC operation, energy consumption prefers mild relative humidity, where relative humidity either too high or low will increase energy consumption with very high sensitivity. Energy consumption is not very sensitive to ambient temperature, slightly in favor of lower temperature. From capture rate or abatement productivity perspective, it strongly in favor of low temperature and mild relative humidity.

The electricity consumption correction after numerical fitting is given by the following, using quadratic equation for temperature $T$ fitting and exponential function for skewed symmetric behavior of relative humidity $RH$:

$$C_t = [1.9 + 0.01(T - 20)](RH - 0.4)^2 e^{RH-0.4} + [1.5 + 0.003(T - 20)^2] \tag{23}$$

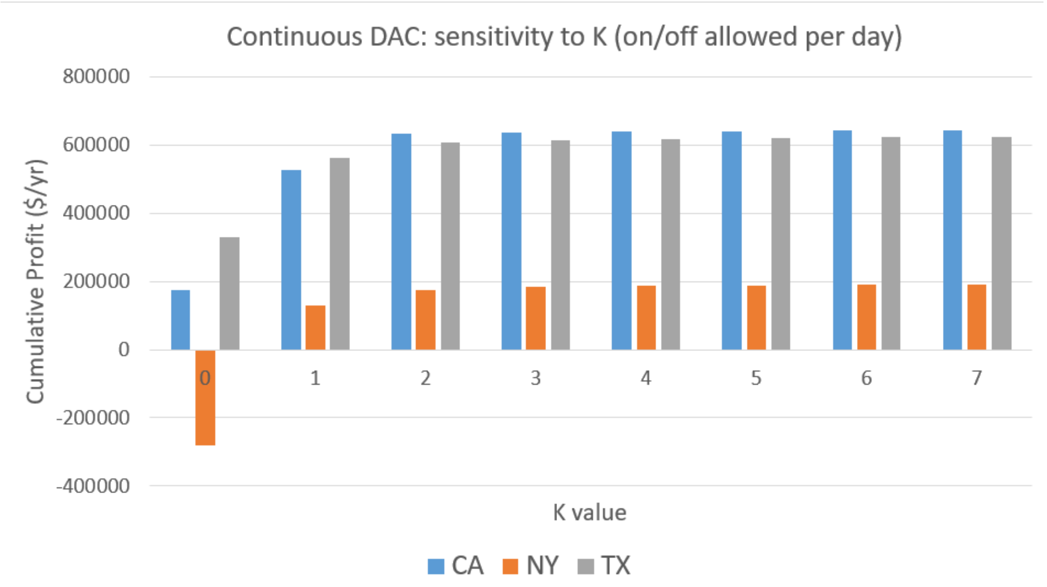


**Fig. S3**: **Sensitivity of profit to flexibility K (turning on/off allowed per day) for continuous DAC operation.** Allowing 2 times of turning on/off is a key flexibility requirement for capturing $\geq 90\%$ of maximum profit from optimization.

The capture rate or abatement correction similarly:

$$\eta_t = 65 - 0.01T^2 - (T + 20)(RH - 0.4)^2 \tag{24}$$

For continuous KOH liquid solvent DAC, capture rate or abatement productivity prefers high temperature and high relative humidity. Little information about energy consumption's sensitivity on ambient conditions. It can be explained by the fact that majoroty of power consumption is used for driving moving equipments and thermal energy for regeneration of solvent at high temperature of 800 °C, both insensitive of ambient conditions.

The capture rate or abatement correction after numerical fitting is given by:

$$\eta_t = 74 + 8(RH - 0.5) + (T - 20) \tag{25}$$

# 2 Data and Processing

NY, CA, and TX data collection and processing are presented, and the processed data input for the model can be accessed from Github Repo.

## 2.1 NY

5-minute resolution NY pricing data for the "MHK VL" zone was downloaded from NYISO's operational data website. This zone was chosen for its high number of industrial facilities, resulting in price fluctuations primarily based on demand.

Emission data was sourced from processing NYISO's Real-Time Fuel Mix data archive, available at a 5-minute resolution for the year 2022. To calculate the Total Adjusted Emission Rate, the Total Demand (MW) was determined by summing up the energy generated from various fuel sources:

$$\text{Total Demand} = \sum_i \text{Demand}_i \tag{26}$$

Where $i$ represents each fuel source.

Using standard emission rates for each fuel type, the Total Emission Rate (TER) for New York was determined by taking the dot product of the energy demand values and the respective emission values, resulting in a weighted sum of the emissions.

$$\text{Total Adjusted Emission Rate} = \frac{\text{TER}}{\text{Total Demand}} \tag{27}$$

The Total Adjusted Emission Rate was then calculated using equation (18).

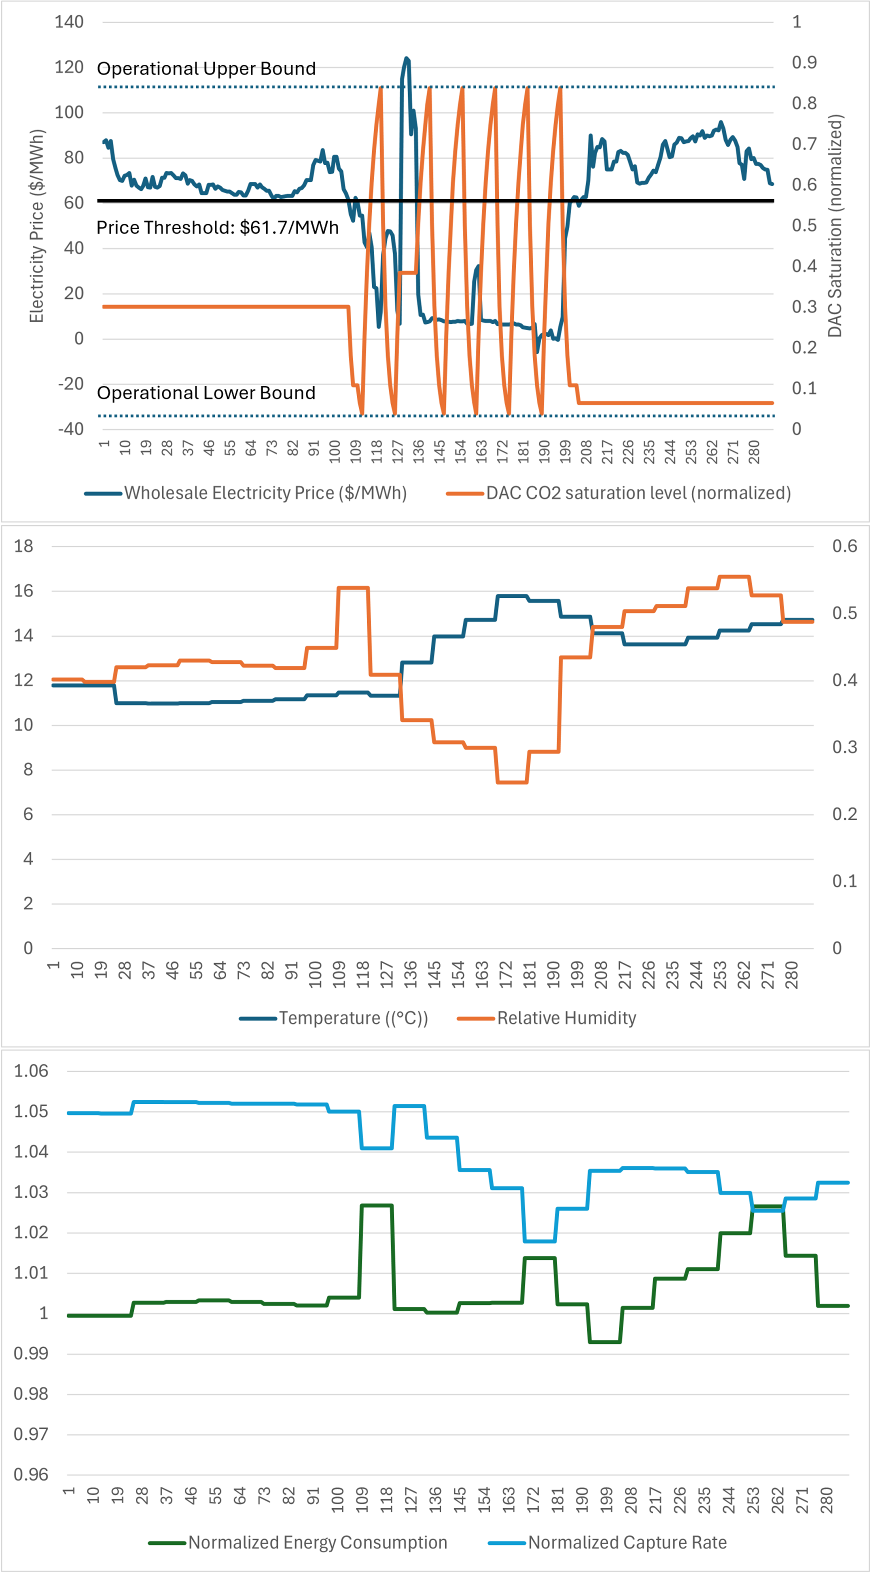


**Fig. S4**: **Representative one-day temporal behavior of DAC operation.** (a) Wholesale electricity price (left axis) and normalized $CO_2$ saturation level (right axis), showing operational bounds and the influence of the bidding threshold. (b) Hourly ambient temperature (left axis) and relative humidity (right axis). (c) Normalized DAC performance metrics—energy consumption efficiency and $CO_2$ capture efficiency—demonstrating the effects of ambient conditions on operational performance and optimization outcomes.

## 2.2 CA

Pricing data was downloaded from CAISO OASIS, capturing 5-minute resolution Locational Marginal Price (LMP) data for the year 2022. The node selected for this study was NEWHALL_1_N001, located in Santa Clarita, California. This area was chosen due to the pronounced representation of the solar "duck curve".

5-min resolution CA emission data (measured in ton-$CO_2$/MWh) was obtained from CAISO's "Today's Outlook". The Total Emission Rate (TER) was then divided by the total demand in MW, sourced from the LMP data, to derive the Total Adjusted Emission Rate.

## 2.3 TX

Texas data from ERCOT using the real-time price (RTP) data and fuel mix data. The TER calculation follows the same formula as NY and CA. This paper uses the price data from "HB WEST" of the ERCOT settlement points in west Texas, this is where the largest ongoing DAC project, STRATOS, is located.

ERCOT has a 15-minute resolution for market clearing. To be consistent with the NY and CA 5-minute resolution comparison, this study reconstructed the 15-minute resolution data to 5-minute resolution by repeating each data point three times, where three 5-minute resolution time steps have the same data to create the 15-minute market clearing interval. For resampling from 15-minute to 5-minute resolution, we apply constant interpolation, repeating each 15-minute price across its three sub-intervals to reflect the fixed market settlement signal. Any missing data from sources are linearly extrapolated from the nearest available data.

## 2.4 Temperature and Relative Humidity Data

| State | Location/Zone | Representative | Lat-1 | Lat-2 | Long-1 | Long-2 | Climate Remarks |
|---|---|---|---|---|---|---|---|
| CA | Santa Clarita | Santa Clarita | 34.5 | 34 | -119 | -118.5 | Hot-summer mediterranean |
| TX | West Texas | Odessa | 32 | 31.5 | -102.5 | -102 | Cold/hot semi-arid |
| NY | MHKVL | Watertown | 44 | 42 | -76 | -74.5 | Warm-summer humid continental |

**Table S2**: Location and description of ambient environmental data collection from Climate Data Store dataset

Ambient environmental data of hourly resolution temperature and relative humidity time series is downloaded from Climate Data Store Climate Data Store "ERA5 pressure levels" based on 1000hPa atmospheric pressure in year 2022 [3]. Details of data description about specific spot data retrieval is in the following table Table S2.

# 3 DAC Power System Model Integration

To better understand the impact of DAC load to power system, both the power price and electricity carbon intensity, an integrated DAC + CAISO power system simulation is added here. The results show that the DAC's scale explored in this study has very limited impact on the overall power system. Even scaled up by $\leq 100$ times, the change of annual power consumption cost is $\leq 5\%$.

The power market model is using the open-sourced model from [4], presenting a Western Electricity Coordinating Council (WECC) power market simulation tool with two-stage market clearing of both day-ahead unit commitment at hourly resolution and real-time price from economic dispatch with 5-min resolution, both consistent with CAISO power market.

To better understand the impact of unpredictable load change due to flexible DAC operation, the DAC load is added to real-time load forecast error instead of base-load that's within the prediction. The DAC load is added to Region 2, where solar duck-curve behavior is most prominent and average power price is similar to historical data. Meanwhile, considering the duck-curve driven DAC operation recovers the solar renewable profile, two different scenarios are generated: (1) DAC scaling without new PV capacity installation; (2) DAC scaling with new PV installation that matches DAC capacity.

The results of DAC power system integration model is presented in Table S3. Due to load added to real-time load forecast error, the day-ahead unit commitment would not see the DAC load and would dispatch the commited generators to satisfy the DAC load, which could be either curtailed

solar PV generation or fossil generators. Therefore, adding PV with DAC load don't always results in lower costs or lower emissions. This problem can be resolved if the DAC load is added to day-ahead load, meaning predictable load. It can be seen that unless DAC is scaled up by 1000 times, meaning 0.8 GW power when turned on, it's impact on it's local locational marginal price and average power carbon intensity is very small, limited within 5%. This proves that using price-taker and carbon-taker assumptions is well defended and very accurate, as the 5% cost gap is smaller than optimization profitability gap from custom algorithm.

| Cases | DAC=1, SR=0 | DAC=10, SR=0 | DAC=100, SR=0 | DAC=1000, SR=0 |
|---|---|---|---|---|
| DAC power costs | +2.3% | +2.5% | +4.6% | +43.7% |
| DAC $CO_2$ emissions | +0.0016% | +0.008% | +0.023% | +0.21% |
| Cases | DAC=1, SR=1 | DAC=10, SR=10 | DAC=100, SR=100 | DAC=1000, SR=1000 |
| DAC power costs | +2.94% | +3.4% | +4.2% | +42.2% |
| DAC power costs | -0.0007% | +0.009% | +0.025% | +0.36% |

**Table S3**: **Strategic operation results of DAC power system integration analysis compared to using price-taker and carbon-taker assumptions.** The cases are named after scaling of DAC. For example, "DAC=10" meaning the DAC is scale up by factor of 10 times as it's modeled in this study; "SR=10" meaning the solar renewable is added by scale of 10. DAC scale of 1 equals to 0.8 MW load on average, solar renewable scale of 1 equals to 2 MW of solar PV.

On the other hand, the integrated simulation with power market model is significantly more computationally expensive. A full year simulation using price-taker and carbon-taker assumptions with custom strategic algorithm takes seconds to solve, while the power market integrated model takes 6-8 hours, mostly repetitively solving unit commitment and economic dispatch optimization. Consider the wide ranges of scenarios and geography coverage in this study include thousands of simulations to run, the power market integrated model is practically impossible. Here we show the results that defend the price-taker and carbon-taker assumptions and all results presented in the manuscript is generated using the assumptions.

# 4 DAC Technology Models

Three different DAC technology samples are extracted from the literature and tested in this study. The details of the technology and parameters for model inputs are summarized in Table S4.

| | SI-AEATPMS | APDES-NFC-FD | MOF |
|---|---|---|---|
| Cycle Switching Cost | 213.36 | 42.02 | 115.60 |
| Adsorption Power Consumption | 0.357 | 0.300 | 0.642 |
| Desorption Power Consumption | 0.071 | 0.060 | 0.097 |
| $\beta_1^a$ | 0.00099 | 0.009434 | 0.2 |
| $\beta_2^a$ | 0 | 0 | -0.2 |
| $\beta_1^d$ | 0 | 0 | 0 |
| $\beta_2^d$ | 0.088 | 0.5 | 0.4 |

**Table S4**: Key Parameters Input for Different DAC Technologies

In this study, two amine-functionalized sorbents, SI-AEATPMS and APDES-NFC-FD, are compared against the Nobel MOF sorbent. Leonzio et al. [5] juxtapose these amine-functionalized sorbents with three Metal-Organic Frameworks (MOFs) - MIL-101, MOF-177, and MOF-5, investigating their efficacy in capturing CO2 from dry air via a temperature swing adsorption system. To get more detailed non-linear adsorption/desorption rates behavior for the MOF sorbent technology, this paper also combined the results from [6][7] to calculate the $\beta$-values.

SI-AEATPMS, which stands for [N-(2-aminoethyl)-3-aminopropyl]trimethoxysilane grafted on silica gel, is created by drying silica gel beads and subsequently loading them with AEATPMS. This technology is characterized by a long, 89.6 hour cycle time, adsorbing for $3.06 \times 10^5$ seconds, and desorbing for $1.67 \times 10^4$ seconds.

Conversely, APDES-NFC-FD, which is 3-aminopropylmethyldiethoxysilane on nanofibrillated cellulose, is made by adding APDES to an NFC hydrogel and then undergoing a freeze-drying process.

This sorbent has a shorter, 9.6 hour cycle time, adsorbing for $3.26 \times 10^4$seconds, and desorbing for $1.85 \times 10^4$ seconds.

It's worth noting that Climeworks, a leading company in the Direct Air Capture (DAC) field, has endorsed these amine-based sorbents. In fact, APDES-NFC-FD is currently being used in their facility in Switzerland.

## 4.1 Parameterization: Translating Source Data to Code Inputs

### 4.1.1 Calculation of Cycle Switching Cost

$S$ represents the total cost per cycle, which is the sum of various operational expenses. It is computed as:

$$S = S_{\text{sorbent material}} + S_{\text{thermal}} \tag{28}$$

### 4.1.2 Calculation of Power Consumption Rates

The power consumption parameters are primarily focused on electrical energy. It's assumed that the regeneration energy is predominantly thermal, which can be sourced at a lower cost from waste heat. The most significant cost component is the electrical energy which is primarily used for fans.

**Adsorption Power Consumption:**

$$P_{\text{a}} = \frac{\text{Total Electricity Consumption (MWh/ton-CO}_2\text{)}}{\text{Number of 5-minute time steps for adsorption}} \tag{29}$$

**Desorption Power Consumption:**

$$P_{\text{d}} = \frac{\text{Total Electricity Consumption (MWh/ton-CO}_2\text{)}}{\text{Number of 5-minute time steps for desorption}} \tag{30}$$

### 4.1.3 Calculation of Beta Coefficients

The beta coefficients, which are used in the piecewise linear approximation for both absorption and desorption, were derived from the figures presented by Leonzio et al.[5] Values were chosen to recover the number of time steps for the desired cycle length. Be minded that to keep consistent across different technologies, these $\beta$-values are calculated using unit capacity where $\bar{X} = 1$.

**Absorption Coefficients:**

For both amine-functionalized sorbents, SI-AEATPMS and APDES-NFC-FD, the adsorption curve figure displays a long flat region before the ratio of outlet to inlet $CO_2$ concentration reaches 1, indicating system saturation. This flat region preceding the breakthrough suggests a linear behavior, which allows for the extrapolation of a linear relationship. Because of this, in the case of SI-AEATPMS and APDES-NFC-FD, the secondary term for the beta values is set to zero:

- $\beta_1^a$: Represents the first-order coefficient for absorption.
- $\beta_2^a$: Represents the second-order coefficient for absorption.

For the calculation of $\beta_1^a$, a line is fit using two distinct points from the figure showing the loading for chemisorbents SI-AEATPMS and APDES-NFC-FD, for both the adsorption rates are effective linear and the second order coefficient is 0.

**Desorption Coefficients:**

For the desorption curve, the behavior is non-linear, so three distinct points from the figure (figure 8) showing CO2 concentration during the desorption step were selected and fit to the equation $X \sim (1 - \beta_2^d)^x$, where $X$ represents the state of saturation, ranging from 0 (completely unsaturated) to 1 (fully saturated). The derived relationship provides the value for $\beta_2^d$.

- $\beta_1^d$: Represents the first-order coefficient for desorption, which is consistently set to zero unless explicitly specified otherwise.
- $\beta_2^d$: Represents the second-order coefficient for desorption derived from the exponential decay fit of the desorption curve.

#### 4.1.4 Calculation of $X_{\text{hat}}$

$X_{\text{hat}}$ represents the maximum capture per one absorption cycle. It is derived from the ratio of the static plant capacity to the number of cycles per year.

The number of cycles per year can be computed as:

$$\text{Number of cycles per year} = \frac{8760}{\text{cycle time (hours)}} \tag{31}$$

Subsequently, $X_{\text{hat}}$ is calculated with:

$$\bar{X} = \frac{100\%\ \text{Plant Capacity}}{\text{Number of cycles per year}} \tag{32}$$

# 5 DAC Sensitivity

Sensitivity analysis based on the previous three DAC technologies is developed, and the details of parameter variation and results are shown in this section.

## 5.1 Sensitivity Tests

**For the Baseline MOF technology:**

- **Cycle cost - low:** Adsorbent part of the overall cycle switching cost reduced to 50% of the original cost.
- **Cycle cost - high:** Adsorbent part of the overall cycle switching cost increased to 200% of the original cost.
- **Energy Efficiency:** Adsorption and desorption power consumption rates reduced by 50% from the original values because the current energy consumption is higher for this technology, thereby offering more scope for improvement in efficiency compared to AP and SI.
- **Cycle duration:** Increased to 400% of the original duration.

**For both AN and SA technologies:**

- **Cycle cost - low:** Adsorbent part of the overall cycle switching cost reduced to 50% of the original cost.
- **Cycle cost - high:** Adsorbent part of the overall cycle switching cost increased to 200% of the original cost.
- **Energy Efficiency:** Adsorption and desorption power consumption rates reduced by 25% from the original values.
- **Cycle duration:** Reduced to 25% of the original duration due to much longer original cycle times.

## 5.2 Design Space Tests

For the purpose of a comprehensive sensitivity analysis, we generated heat maps by running the MATLAB code for DAC optimization across a range of cycle times and cycle costs. The specifics of these parameter sets are as follows:

- **Cycle Time:** The cycle time was varied across 22 values, increasing exponentially by a factor of $2^{\frac{1}{3}}$ from 1 to 128 hours:

$$1, 1.26, 1.59, 2, 2.52, \ldots, 50.79, 64, 80.64, 101.59, 128$$

- **Cycle Cost:** The cycle cost was varied across 17 values, again increasing exponentially by a factor of $2^{\frac{1}{3}}$ from 10 to 402.65 USD:

$$10, 12.60, 15.88, 20.00, 25.20, \ldots, 160.00, 201.58, 253.96, 320.00, 402.65$$

Upon specifying the range for cycle times and costs, matrices were initialized to store the results pertaining to both profit and $CO_2$ values.
The code then iterates through each combination of cycle time and cycle cost. For each combination the parameters were altered to match the given cycle cost and cycle time as shown below:

**Table S5**: Sensitivity Analysis for Different DAC Technologies

| | Variation | SI-AEATPMS | APDES-NFC-FD | Baseline (MOF) |
|---|---|---|---|---|
| $\bar{X}$ | Baseline | 23.95 | 2.64 | 1 |
| | Cycle Cost - Low | 23.95 | 2.64 | 1 |
| | Cycle Cost - High | 23.95 | 2.64 | 1 |
| | Energy Efficiency | 23.95 | 2.64 | 1 |
| | Cycle Length | 5.99 | 0.66 | 4 |
| Cycle Switching Cost | Baseline | 213.36 | 42.02 | 115.60 |
| | Cycle Cost - Low | 129.36 | 38.17 | 95.60 |
| | Cycle Cost - High | 381.36 | 49.72 | 155.60 |
| | Energy Efficiency | 213.36 | 42.02 | 115.60 |
| | Cycle Length | 213.36 | 42.02 | 115.60 |
| Adsorption Power Consumption ($P_{\text{a\_unit}}$) | Baseline | 0.000353 | 0.002830 | 0.080250 |
| | Cycle Cost - Low | 0.000353 | 0.002830 | 0.080250 |
| | Cycle Cost - High | 0.000353 | 0.002830 | 0.080250 |
| | Energy Efficiency | 0.000265 | 0.002123 | 0.040125 |
| | Cycle Length | 0.001414 | 0.011321 | 0.020063 |
| Desorption Power Consumption ($P_{\text{d\_unit}}$) | Baseline | 0.001427 | 0.008571 | 0.016167 |
| | Cycle Cost - Low | 0.001427 | 0.008571 | 0.016167 |
| | Cycle Cost - High | 0.001427 | 0.008571 | 0.016167 |
| | Energy Efficiency | 0.001065 | 0.006429 | 0.008083 |
| | Cycle Length | 0.005680 | 0.034286 | 0.004042 |
| $\beta_1^a$ | Baseline | 0.00099 | 0.009434 | 0.2 |
| | Cycle Cost - Low | 0.00099 | 0.009434 | 0.2 |
| | Cycle Cost - High | 0.00099 | 0.009434 | 0.2 |
| | Energy Efficiency | 0.00099 | 0.009434 | 0.2 |
| | Cycle Length | 0.00396 | 0.037736 | 0.05 |
| $\beta_2^a$ | Baseline | 0 | 0 | -0.2 |
| | Cycle Cost - Low | 0 | 0 | -0.2 |
| | Cycle Cost - High | 0 | 0 | -0.2 |
| | Energy Efficiency | 0 | 0 | -0.2 |
| | Cycle Length | 0 | 0 | -0.05 |
| $\beta_1^d$ | Baseline | 0 | 0 | 0 |
| | Cycle Cost - Low | 0 | 0 | 0 |
| | Cycle Cost - High | 0 | 0 | 0 |
| | Energy Efficiency | 0 | 0 | 0 |
| | Cycle Length | 0 | 0 | 0 |
| $\beta_2^d$ | Baseline | 0.088 | 0.5 | 0.4 |
| | Cycle Cost - Low | 0.088 | 0.5 | 0.4 |
| | Cycle Cost - High | 0.088 | 0.5 | 0.4 |
| | Energy Efficiency | 0.088 | 0.5 | 0.4 |
| | Cycle Length | 0.352 | 2 | 0.1 |
| Increment and Look Ahead | Baseline | 3211 | 343 | 288 |
| | Cycle Cost - Low | 3211 | 343 | 288 |
| | Cycle Cost - High | 3211 | 343 | 288 |
| | Energy Efficiency | 3211 | 343 | 288 |
| | Cycle Length | 803 | 288 | 288 |

1. $X_{\textbf{hat}}$**:** Given the static plant capacity (*Capacity*) and the total hours in a year (8760), $X_{\text{hat}}$ is calculated using the formula:
$$\bar{X} = \frac{Capacity}{\frac{8760}{\text{cycle\_time}}}$$
2. **Switching Cost** $S$**:** This is determined by multiplying $\bar{X}$ with the cycle cost:
$$S = \bar{X} \times \text{cycle\_cost}$$
3. **Power Consumption for Adsorption (** $P_{\textbf{a\_unit}}$ **):** Given the baseline power consumption rate ($P_{a-raw}$) and the number of 5-min adsorption time steps ($n_a$), the adjusted power consumption rate is:
$$P_{\text{a\_unit}} = \frac{P_{a-raw}}{n_a}$$

4. **Power Consumption for Desorption ( $P_{\mathbf{d\_unit}}$ ):** Similarly, the power consumption rate for desorption is:

$$P_{\text{d\_unit}} = \frac{P_{d-raw}}{n_d}$$

5. **Total Power Consumption:** The total power consumption for both adsorption and desorption are then:

$$P_a = P_{\text{a\_unit}} \times \bar{X}$$
$$P_d = P_{\text{d\_unit}} \times \bar{X}$$

6. **Beta Coefficients:** Using the baseline coefficients where $\bar{X}$=1, the adjusted beta coefficients are determined as following and will be eventually adopted for final parameter input for code:

$$\beta^a_{1-adjust} = \beta^a_1 \cdot \bar{X}$$
$$\beta^a_{2-adjust} = \beta^a_2$$
$$\beta^d_{1-adjust} = \beta^d_1 \cdot \bar{X}$$
$$\beta^d_{2-adjust} = \beta^d_2$$

7. **Increment and Look-Ahead Adjustments:** Depending on the cycle time, the increment and look-ahead values are adjusted:
   - If cycle_time < 8 hours, both increment and look-ahead are set to 288 time steps (24 hours).
   - Otherwise, the factor is determined by cycle_time/8, and both increment and look-ahead are set to 288 × factor.

# 6 Supplementary Results and Discussions

## 6.1 Temporal behavior discussion

In the main text, Fig. 2(c), there exists a mismatch between the price peak in July and $CO_2$ removal valley in August for TX. This is due to the aggregated results from daily to monthly that masked some outliers' impact. Here we provide a 2 month and also 1 day zoom in for these detailed temporal behaviors in S3. In July, the high average price is driven by some significantly expensive days while there are still 8 days with the average price lower than \$60/MWh, which makes the DAC operation marginally profitable during these days, therefore maintaining a moderate DAC capacity factor. In August, although the average price is much lower than in July since it does not have any extreme outliers, all 31 days in August have a price higher than \$60/MWh, making the DAC not profitable, and DAC operation is only viable during some exceptional hours on certain days, leading to a very low capacity factor. This mismatch introduced by aggregating higher temporal resolution results to lower resolution is another solid proof that increasing temporal resolution can gain higher profit and is more informative to DAC operators. Using average electricity properties can be misleading in some cases, either using annual, monthly, or even daily average for operation scheduling. It highlights the importance of high temporal resolution analysis, especially considering power market volatility.

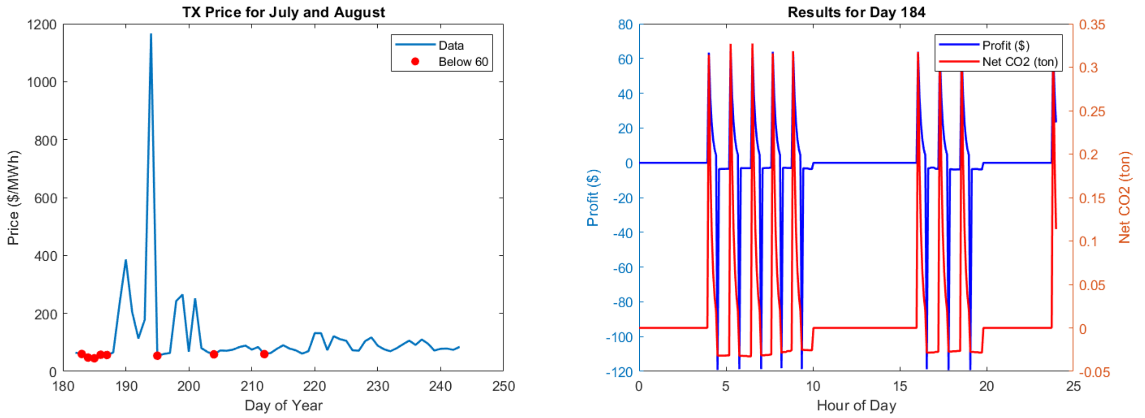


**Fig. S5: TX detailed zoom in for (left) July and August daily price profile and (right) 1-day zoom DAC dynamic behavior profile with profit and net $CO_2$ captured.** Negative net-$CO_2$ captured means adsorption process consumes electricity and have net-$CO_2$ emissions. We can clearly see the cyclic behavior of MOF DAC system with roughly 1 hour cycle time.

## 6.2 Sensitivity analysis results

Figures S6 to Figures S11 showing the results for the sensitivity tests.

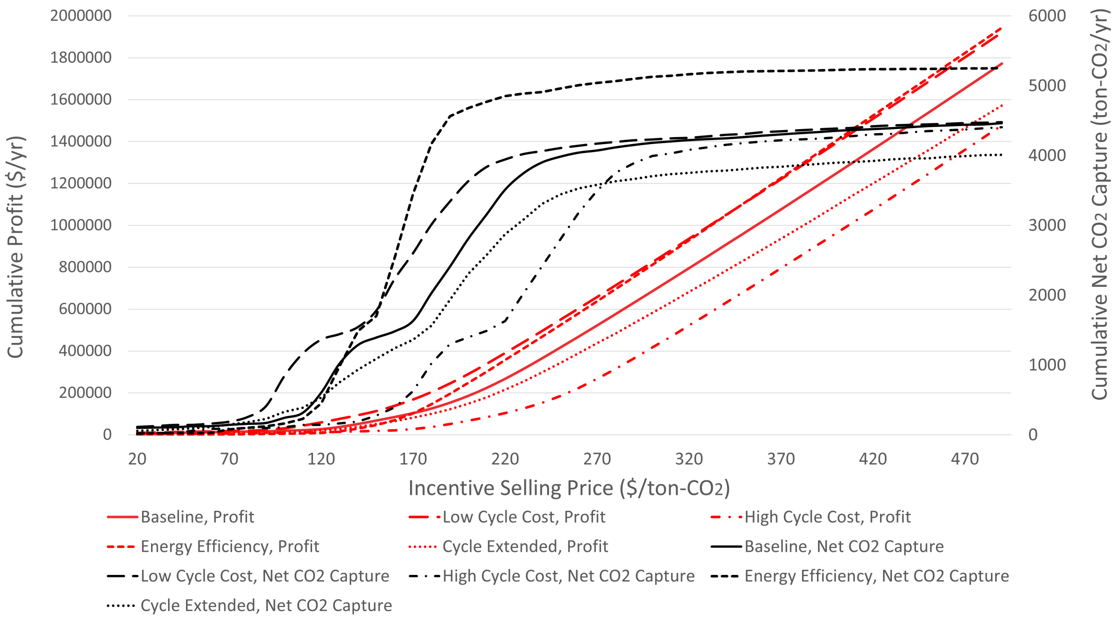


**Fig. S6: Sensitivity analysis for MOF technology: wholesale electricity price case.**

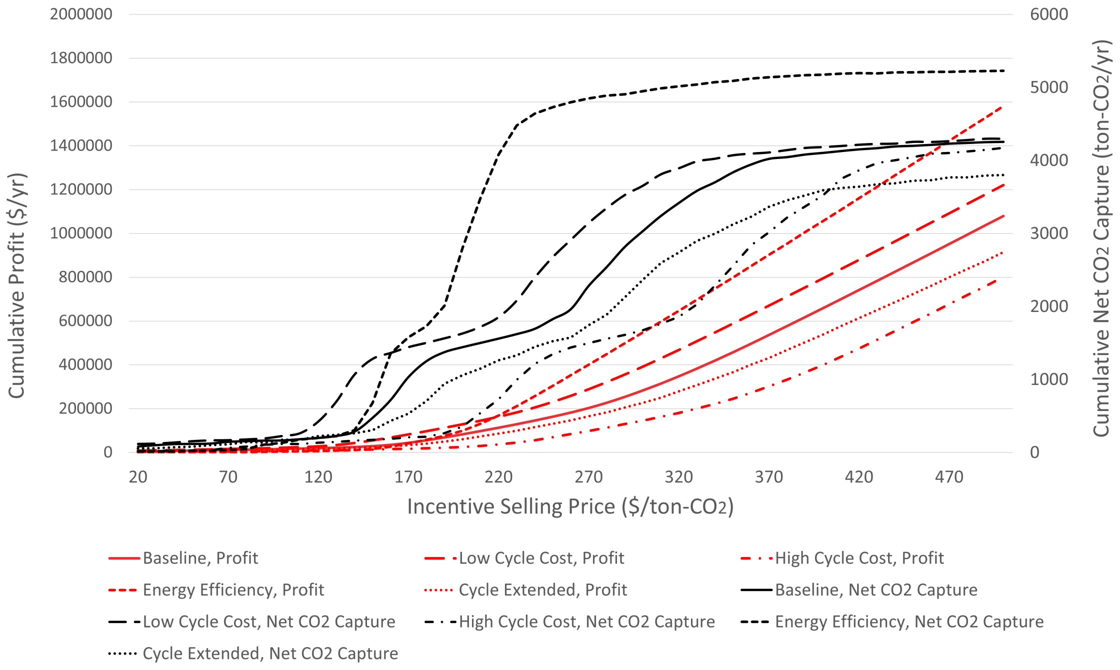


**Fig. S7**: **Sensitivity analysis for MOF technology: carbon-tax adjusted price case.**

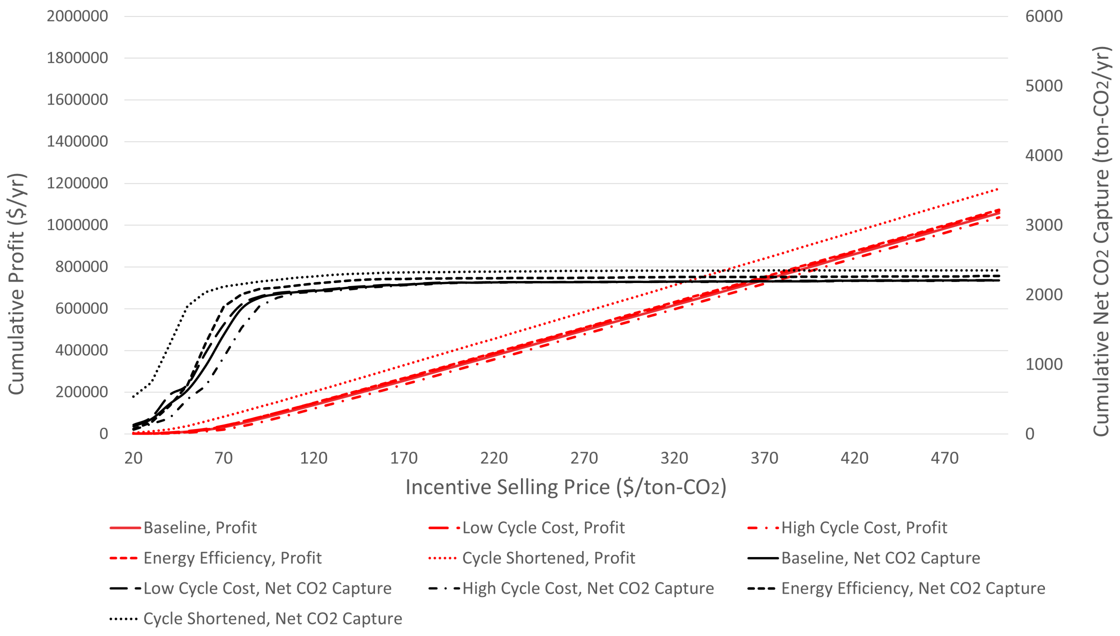


**Fig. S8**: **Sensitivity analysis for AN technology: wholesale electricity price case.**

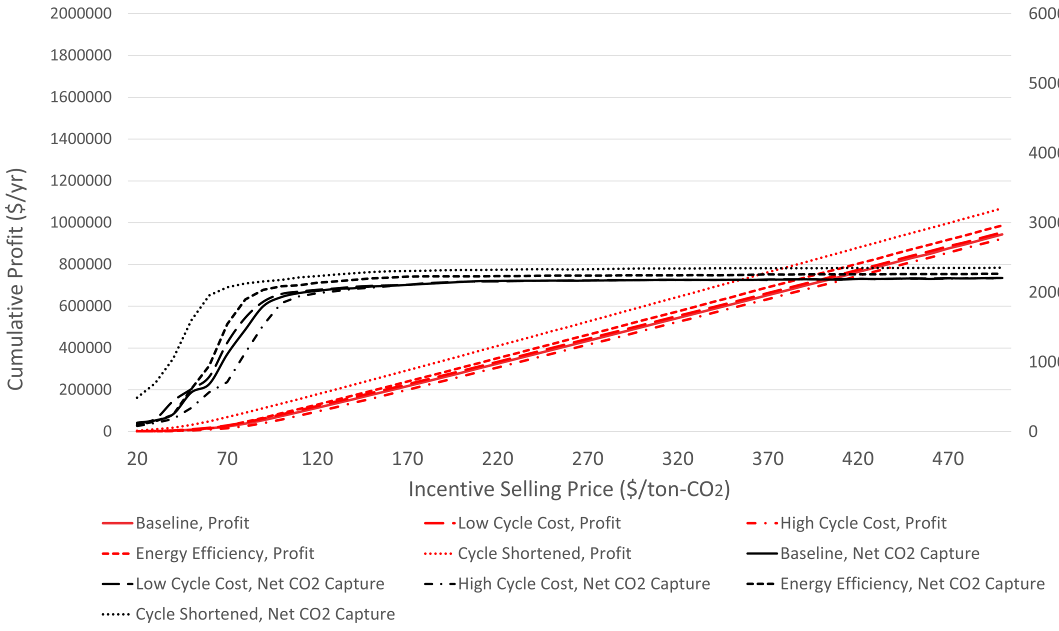


**Fig. S9**: **Sensitivity analysis for AN technology: carbon-tax adjusted price case.**

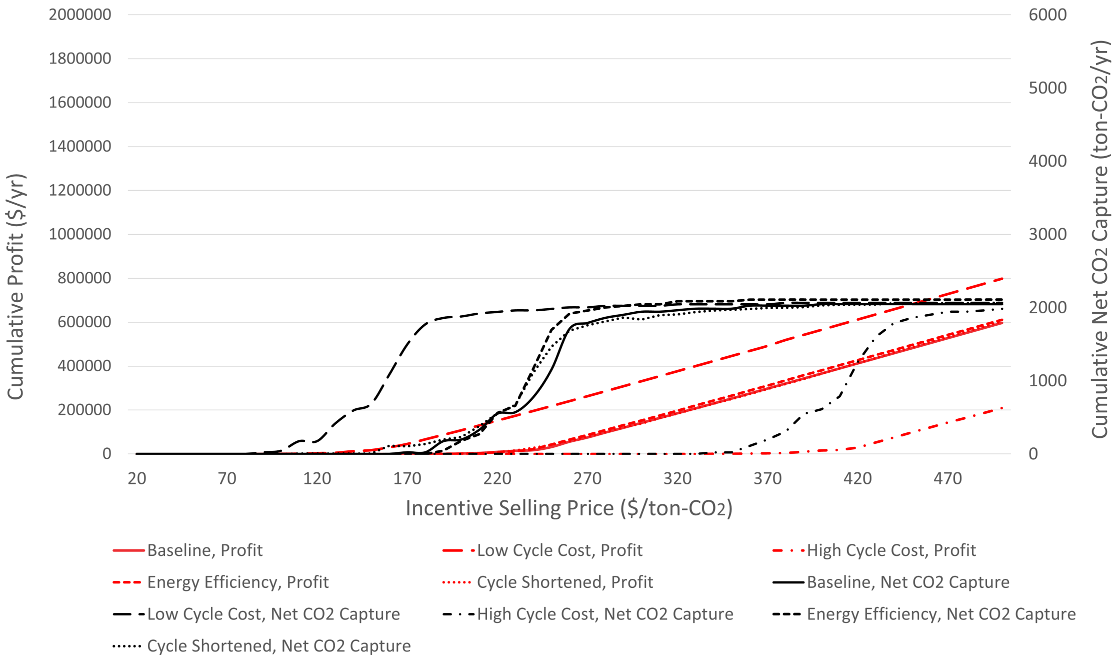


**Fig. S10**: **Sensitivity analysis for SA technology: wholesale electricity price case.**

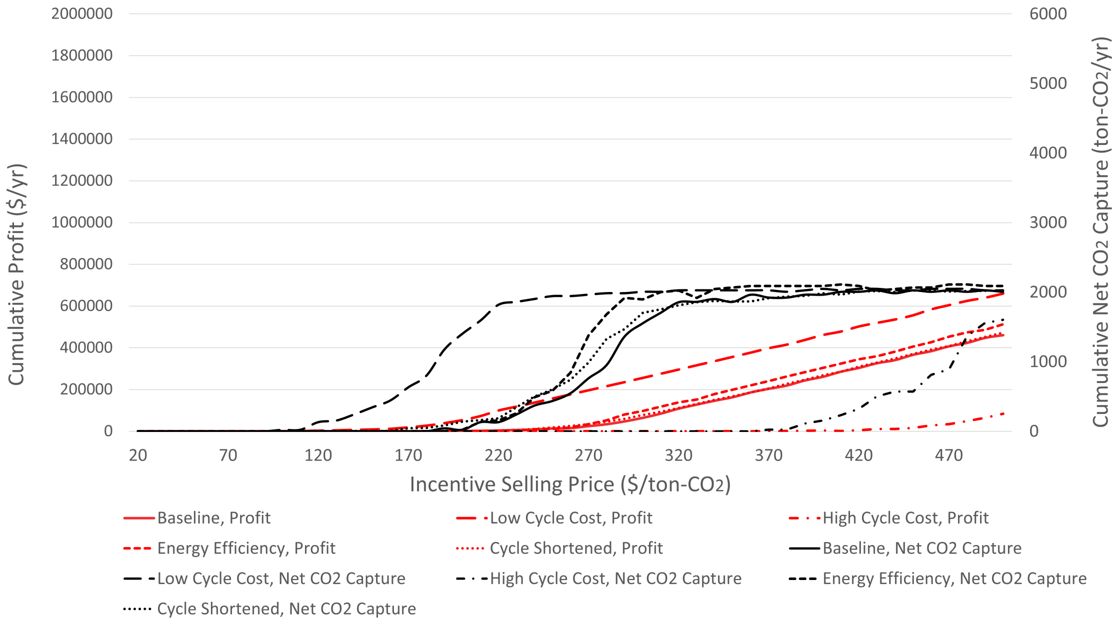


**Fig. S11**: **Sensitivity analysis for SA technology: carbon-tax adjusted price case.**

# References

[1] Sendi, M., Bui, M., Mac Dowell, N., Fennell, P.: Geospatial analysis of regional climate impacts to accelerate cost-efficient direct air capture deployment. One Earth **5**(10), 1153–1164 (2022) https://doi.org/10.1016/j.oneear.2022.09.003 . Accessed 2024-04-08

[2] An, K., Farooqui, A., McCoy, S.T.: The impact of climate on solvent-based direct air capture systems. Applied Energy **325**, 119895 (2022) https://doi.org/10.1016/j.apenergy.2022.119895 . Accessed 2024-04-08

[3] Copernicus Climate Change Service: ERA5 hourly data on pressure levels from 1940 to present. Copernicus Climate Change Service (C3S) Climate Data Store (CDS) (2018). https://doi.org/10.24381/CDS.BD0915C6 . https://cds.climate.copernicus.eu/doi/10.24381/cds.bd0915c6 Accessed 2024-12-08

[4] Zheng, N., Xu, B.: A WECC-based Model for Simulating Two-stage Market Clearing with High-temporal-resolution. arXiv. Version Number: 1 (2023). https://doi.org/10.48550/ARXIV.2312.15349 . https://arxiv.org/abs/2312.15349 Accessed 2024-11-06

[5] Leonzio, G., Mwabonje, O., Fennell, P.S., Shah, N.: Environmental performance of different sorbents used for direct air capture. Sustainable Production and Consumption **32**, 101–111 (2022) https://doi.org/10.1016/j.spc.2022.04.004 . Accessed 2023-10-31

[6] Azarabadi, H., Lackner, K.S.: A sorbent-focused techno-economic analysis of direct air capture. Applied Energy **250**, 959–975 (2019) https://doi.org/10.1016/j.apenergy.2019.04.012 . Accessed 2023-10-31

[7] Sinha, A., Darunte, L.A., Jones, C.W., Realff, M.J., Kawajiri, Y.: Systems Design and Economic Analysis of Direct Air Capture of $CO_2$ through Temperature Vacuum Swing Adsorption Using MIL-101(Cr)-PEI-800 and mmen-$Mg_2$ (dobpdc) MOF Adsorbents. Industrial & Engineering Chemistry Research **56**(3), 750–764 (2017) https://doi.org/10.1021/acs.iecr.6b03887 . Accessed 2023-05-26
